# Supplementary material for: Simulating User Satisfaction for the Evaluation of Task-oriented Dialogue Systems
Source: arXiv:2105.03748 source file (2021-05-08)
Supplement: Supplementary file 1 [file 09_Appendix.tex]

% \section{Cross-domain analysis}

% Since we have multiple domains in the dataset, we further analyze the cross-domain generalization capabilities of the user satisfaction prediction model (We did not test JDDC because the language of JDDC is different from other data.). Table.\ref{appendix:table:cross-domain} shows the results. The rows and columns in Table.\ref{appendix:table:cross-domain} indicate training data and test data, respectively (eg. 0.233 in the first column of the sixth row indicates that a BERT model trained on MultiWOZ can get a UAR score of 0.233 on SGD data.). 
% In terms of data sets, the models trained on SGD and MultiWOZ get the best performance on each other’s data respectively, and the models trained on ReDial get the best performance on CCPE, possibly due to the similarity between domains. The model trained on CCPE has relatively poor generalization ability, possibly due to limited less training data size.
% In terms of methods, BERT achieves better generalization performance than SVM and HiGRU, possibly due to the improvement of pre-training on the large-scale corpus.
% % =========================================
% % Cross-domain results
% % =========================================
% \begin{table}[]
% \centering
% % \setlength\tabcolsep{2pt}
% \caption{Cross-domain performance for user satisfaction prediction. Report UAR.}
% \label{appendix:table:cross-domain}
% \begin{tabular}{ll cccc}
% \toprule
% \textbf{From} & \textbf{To}
% & \textbf{SGD}  & \textbf{MWOZ} & \textbf{ReDial}  & \textbf{CCPE}
% \\

% \midrule
% \multirow{2}{*}{\textbf{SGD}}
% & SVM
% & \textcolor{gray}{0.230}     & 0.209   & 0.211  & 0.198
% \\
% & HiGRU
% & \textcolor{gray}{0.293}     & 0.240   & 0.230  & 0.212
% \\
% & BERT
% & \textcolor{gray}{0.261}     & \textbf{0.249}   & \textbf{0.254}  & 0.223
% \\
% \midrule
% \multirow{2}{*}{\textbf{MWOZ}}
% & SVM
% & 0.208     & \textcolor{gray}{0.215}   & 0.206  & 0.208
% \\
% & HiGRU
% & 0.224     & \textcolor{gray}{0.225}   & 0.221  & 0.219
% \\
% & BERT
% & \textbf{0.233}     & \textcolor{gray}{0.256}   & 0.219  & 0.226
% \\
% \midrule
% \multirow{2}{*}{\textbf{ReDial}}
% & SVM
% & 0.216     & 0.227   & \textcolor{gray}{0.221}  & 0.199
% \\
% & HiGRU
% & 0.211     & 0.221   & \textcolor{gray}{0.261}  & 0.220
% \\
% & BERT
% & 0.228     & 0.218   & \textcolor{gray}{0.257}  & \textbf{0.239}
% \\
% \midrule
% \multirow{2}{*}{\textbf{CCPE}}
% & SVM
% & 0.217     &  0.208   & 0.218  & \textcolor{gray}{0.214}
% \\
% & HiGRU
% & 0.211     & 0.223   & 0.227  & \textcolor{gray}{0.237}
% \\
% & BERT
% & 0.216     & 0.213   & 0.219  & \textcolor{gray}{0.232}
% \\
% \bottomrule
% \end{tabular}

% \end{table}

% % END Cross-domain results ============================================

% \section{Taxonomies of JDDC user action}
% \label{appendix:jddc}
